# Supplementary material for: SceneWiz3D: Towards Text-guided 3D Scene Composition
Source: arXiv:2312.08885 source file (2023-12-13)
Supplement: Supplementary file 1 [file supp.tex]

% CVPR 2024 Paper Template; see https://github.com/cvpr-org/author-kit

\documentclass[10pt,twocolumn,letterpaper]{article}

%%%%%%%%% PAPER TYPE  - PLEASE UPDATE FOR FINAL VERSION
% \usepackage{cvpr}              % To produce the CAMERA-READY version
\usepackage[review]{cvpr}      % To produce the REVIEW version
% \usepackage[pagenumbers]{cvpr} % To force page numbers, e.g. for an arXiv version

% Import additional packages in the preamble file, before hyperref
\usepackage{float}
\usepackage{booktabs,multirow,adjustbox,diagbox,threeparttable}
\usepackage{capt-of}
\usepackage{wrapfig}
\input{preamble}
\usepackage{times}
\usepackage{xcolor}
\usepackage{xspace}
\usepackage{capt-of}
\usepackage{wrapfig}
\usepackage{graphicx}
\usepackage{amsmath,amssymb,amsfonts,dsfont,pifont,bm,bbm,mathrsfs,mathtools,nicefrac}
\usepackage{algorithm,algpseudocode,listings}
\usepackage{booktabs,multirow,adjustbox,diagbox,threeparttable}
\usepackage{animate}
\definecolor{citeblue}{RGB}{48,111,186}
\usepackage[pagebackref=false,breaklinks=true,colorlinks=true,citecolor=citeblue,bookmarks=false]{hyperref}
\usepackage{capt-of}
\usepackage{wrapfig}
\usepackage{paralist}
% It is strongly recommended to use hyperref, especially for the review version.
% hyperref with option pagebackref eases the reviewers' job.
% Please disable hyperref *only* if you encounter grave issues, 
% e.g. with the file validation for the camera-ready version.
%
% If you comment hyperref and then uncomment it, you should delete *.aux before re-running LaTeX.
% (Or just hit 'q' on the first LaTeX run, let it finish, and you should be clear).
\definecolor{cvprblue}{rgb}{0.21,0.49,0.74}
\usepackage[pagebackref,breaklinks,colorlinks,citecolor=cvprblue]{hyperref}

\usepackage{xspace}

%% external package
\usepackage[utf8]{inputenc}
\usepackage{booktabs}
\usepackage{bm}
% \usepackage{amsmath}  

%%%%%%%%% PAPER ID  - PLEASE UPDATE
 % *** Enter the Paper ID here

%%%%%%%%% TITLE - PLEASE UPDATE

\title{Towards Text-guided 3D Scene Composition}

%%%%%%%%% AUTHORS - PLEASE UPDATE
\author{
% First Author\\
% Institution1\\
% Institution1 address\\
% {\tt\small firstauthor@i1.org}
% % For a paper whose authors are all at the same institution,
% % omit the following lines up until the closing ``}''.
% % Additional authors and addresses can be added with ``\and'',
% % just like the second author.
% % To save space, use either the email address or home page, not both
% \and
% Second Author\\
% Institution2\\
% First line of institution2 address\\
% {\tt\small secondauthor@i2.org}
}

\begin{document}

% \twocolumn[{
% \renewcommand\twocolumn[1][]{#1}
\maketitle
% \begin{center}
% \includegraphics[width=1\linewidth,clip, trim=0 0 0 0]{fig/teaser.pdf}
%   \captionsetup{type=figure,font=small}
%   \vspace{-5mm}
%   \caption{Diverse individual scenes and large-scale scenes generated by \NAME. The generated scene is represented by the semantic occupancy map, where the color labels indicate different semantic categories. The input BEV layout is also attached as a reference.} 
%   \label{fig:teaser}
%   \vspace{5pt}
% \end{center}
% }]

\thispagestyle{empty}

\input{sec/X_suppl}
{
    \small
    \bibliographystyle{ieeenat_fullname}
    \bibliography{main}
}

% WARNING: do not forget to delete the supplementary pages from your submission 

\end{document}
